# Supplementary material for: Long Working Distance Apodized Grating Coupler
Source: arXiv:2006.16247 source file (2020-06-29)
Supplement: Supplementary file 1 [file appendice.tex]

\section*{Fiber Numerical Aperture (NA) in Radians}
	\label{sec:numerical_aperture}
	
	Numerical aperture of a standard single mode fiber (SMF) measured at $1 \%$ power level of an 1D far-field scan at 1550 nm is $0.14$. At $1 \%$ power level of the Gaussian output beam $ exp ( - 2 (\frac{w_{1 \%}}{\sigma})^2 ) = 0.01$ where $w_{1 \%}$ is the half beam width. At the half of the maximum power level $  exp ( - 2 (\frac{w_{FWHM}/2}{\sigma}) ^2 ) = 1/2 $ where $w_{FWHM}$ is the full width at the half of maximum power. We can readily obtain that $w_{1 \%} = \sigma$ and $w_{FWHM} = \sigma \sqrt{2ln(2)}$. Width at one percent power level is related to the  $w_{FWHM}$ by the factor $\frac{w_{FWHM}}{w_{1 \%}} = sqrt{\frac{2ln(2)}{ln(10)}} = 0.775925$.  To match the fiber mode, the output beam from the grating should achieve the full width  $w_{FWHM} \sim 0.1$ radians.
